# Supplementary material for: Estimating Feature-Label Dependence Using Gini Distance Statistics
Source: arXiv:1906.02171 source file (2019-06-05)
Supplement: Supplementary file 1 [file appendices.tex]

\documentclass[10pt,final,twocolumn,compsoc]{IEEEtran}
% Some very useful LaTeX packages include:
% (uncomment the ones you want to load)

% *** CITATION PACKAGES ***
%
\ifCLASSOPTIONcompsoc
  % IEEE Computer Society needs nocompress option
  % requires cite.sty v4.0 or later (November 2003)
  \usepackage[nocompress]{cite}
\else
  % normal IEEE
  \usepackage{cite}
\fi

% *** MATH PACKAGES ***
%
\usepackage{amsmath}
% A popular package from the American Mathematical Society that provides
% many useful and powerful commands for dealing with mathematics.
%
% Note that the amsmath package sets \interdisplaylinepenalty to 10000
% thus preventing page breaks from occurring within multiline equations. Use:
%\interdisplaylinepenalty=2500
% after loading amsmath to restore such page breaks as IEEEtran.cls normally
% does. amsmath.sty is already installed on most LaTeX systems. The latest
% version and documentation can be obtained at:
% http://www.ctan.org/pkg/amsmath
\usepackage{amsfonts}
\usepackage{amssymb}
\usepackage{amsthm}
\usepackage{eqnarray}
\usepackage{graphicx}
\usepackage{caption}
\usepackage{multirow}

\newtheorem{thm}{Theorem}

% correct bad hyphenation here
\hyphenation{op-tical net-works semi-conduc-tor}

\begin{document}
\title{Estimating Feature-Label Dependence Using Gini Distance Statistics}

\author{Silu Zhang,
        Xin Dang,~\IEEEmembership{Member,~IEEE,}
        Dao Nguyen,
        Dawn Wilkins,~Yixin Chen,~\IEEEmembership{Member,~IEEE}% <-this % stops a space
% \IEEEcompsocitemizethanks{\IEEEcompsocthanksitem S. Zhang, D. Wilkins, and Y. Chen are with the Department of Computer and Information Science. X. Dang and D. Nguyen are with the Department of Mathematics, University of Mississippi, University, MS 38677, USA. E-mail: \{szhang6,xdang,dxnguyen,dwilkins,yixin\}@olemiss.edu
% %\protect\\
% % note need leading \protect in front of \\ to get a newline within \thanks as
% % \\ is fragile and will error, could use \hfil\break instead.
% %\IEEEcompsocthanksitem B and C are with University of Mississippi.
% }% <-this % stops an unwanted space
% %\thanks{Manuscript received April 19, 2005; revised August 26, 2015.}
}

% The paper headers
\markboth{IEEE Transactions on Pattern Analysis and Machine Intelligence,~Vol.~, No.~, ~2019}
{Estimating Feature-Label Dependence Using Gini Distance Statistics}
% The only time the second header will appear is for the odd numbered pages
% after the title page when using the twoside option.
% 
% *** Note that you probably will NOT want to include the author's ***
% *** name in the headers of peer review papers.                   ***
% You can use \ifCLASSOPTIONpeerreview for conditional compilation here if
% you desire.

% make the title area
\maketitle

% To allow for easy dual compilation without having to reenter the
% abstract/keywords data, the \IEEEtitleabstractindextext text will
% not be used in maketitle, but will appear (i.e., to be "transported")
% here as \IEEEdisplaynontitleabstractindextext when the compsoc 
% or transmag modes are not selected <OR> if conference mode is selected 
% - because all conference papers position the abstract like regular
% papers do.
\IEEEdisplaynontitleabstractindextext
% \IEEEdisplaynontitleabstractindextext has no effect when using
% compsoc or transmag under a non-conference mode.

% For peer review papers, you can put extra information on the cover
% page as needed:
% \ifCLASSOPTIONpeerreview
% \begin{center} \bfseries EDICS Category: 3-BBND \end{center}
% \fi
%
% For peerreview papers, this IEEEtran command inserts a page break and
% creates the second title. It will be ignored for other modes.
\IEEEpeerreviewmaketitle

\newpage
\appendices
\section{Proof of Lemma 1}\label{app_a}
\begin{proof}
From (8), we write
\begin{equation}\label{ABC}\tag{27}
    \mathrm{dCov}_{\kappa_X,\kappa_Y}(X,Y) = A + B - 2C,
\end{equation}
where
\begin{align*}
A&=\mathbb{E}d_{\kappa_X}(X,X')d_{\kappa_Y}(Y,Y'),\\
B&=\mathbb{E}d_{\kappa_X}(X,X')\mathbb{E}d_{\kappa_Y}(Y,Y'),\\
C&=\mathbb{E}\left[\mathbb{E}_{X'}d_{\kappa_X}(X,X')\mathbb{E}_{Y'}d_{\kappa_Y}(Y,Y')\right].
\end{align*}
Then we have
\begin{align}
    A & = \sum_{i\ne j}{\int_{\mathbb{R}^{2q}}p_ip_j d_{\kappa_X}(x,x')dF_i\times F_j} \nonumber\\
      %& = \sum_{i,j}{\int_{\mathbb{R}^{2q} }p_ip_j d_{\kappa_X}(x,x')dF_i\times F_j} - \sum_{k}{\int_{\mathbb{R}^{2q}}p_k^2 d_{\kappa_X}(x,x')dF_k\times F_k}\nonumber\\
      & = \int_{\mathbb{R}^{2q}} d_{\kappa_X}(x,x')dF \times F \nonumber\\
      & - \sum_{k}{p_k^2\int_{\mathbb{R}^{2q}} d_{\kappa_X}(x,x')dF_k\times F_k} \nonumber\\
      & = \mathbb{E} d_{\kappa_X}(X,X') - \sum_k{p_k^2 \mathbb{E}d_{\kappa_X}(X_k,{X_k}')},\label{A}\tag{28}\\
% \end{align}
% \begin{align}
     B & = \mathbb{E}d_{\kappa_X}(X,X') \left( 1 - \sum_{k}{p_k^2} \right) \nonumber\\
      & = \mathbb{E} d_{\kappa_X}(X,X') - \sum_k p_k^2 \mathbb{E}{d_{\kappa_X}(X,X')},\label{B}\tag{29}
\end{align}
\begin{align}
    C & = \mathbb{E}_{Y}\left[ \mathbb{E}_{X|Y} \int_{\mathbb{R}^q} d_{\kappa_X}(x,x')dF \cdot \sum_{k'}{p_{k'}d_{\kappa_Y}(Y,k')} \right] \nonumber\\
      & = \mathbb{E}_{Y} \left[ \int_{\mathbb{R}^{2q}} d_{\kappa_X}(x,x')dF \times F_Y \cdot \sum_{k'}{p_{k'}d_{\kappa_Y}(Y,k')} \right] \nonumber\\
      & = \sum_{k \ne k'}{\int_{\mathbb{R}^{2q}} d_{\kappa_X}(x,x')p_k p_{k'} dF \times F_k} \nonumber\\
    %   & = \sum_{k,k'}{\int_{\mathbb{R}^{2q}} d_{\kappa_X}(x,x')p_k p_{k'} dF \times F_k} - \sum_{k}{\int_{\mathbb{R}^{2q}} d_{\kappa_X}(x,x')p_k^2 dF \times F_k} \nonumber\\
      & = \sum_{k}{\int_{\mathbb{R}^{2q}} d_{\kappa_X}(x,x')p_k dF \times F_k} - \sum_{k}{p_k^2 \mathbb{E} d_{\kappa_X}(X_k,X)} \nonumber\\
    %  & = \int_{\mathbb{R}^{2q}} d_{\kappa_X}(x,x') dF \times F - \sum_{k}{p_k^2 \mathbb{E} d_{\kappa_X}(X_k,X)} \nonumber\\
      & = \mathbb{E}d_{\kappa_X}(X,X') - \sum_{k}{p_k^2 \mathbb{E}d_{\kappa_X}(X_k,X)}.\label{C}\tag{30}
\end{align}
The proof is completed by substituting (\ref{A}), (\ref{B}), and (\ref{C}) into (\ref{ABC}).
\end{proof}

\section{Proof of the uniform convergence bounds}\label{app_b}
\begin{thm}[\bf McDiarmid's Inequality]
Let $X_1,X_2,\dots,X_n$ be independent random variables taking values in a set ${\mathbb X}$. Let $f:{\mathbb X}^n \rightarrow {\mathbb R}$ be a function of $X_1,X_2,\dots,X_n$ that satisfies
% $$ 
% \sup_{x_1,\dots, x_n, \hat{x}_i \in {\mathbb X}} |f(x_1,\dots,x_n) - f(x_1,\dots,x_{i-1},\hat{x}_i, x_{i+1},\dots, x_n)| \le c_i,
% $$
$$ 
\sup_{x_1,\dots, x_n, \hat{x}_i \in {\mathbb X}} |f(x_1,\dots,x_n) - f(x_1,\dots,\hat{x}_i,\dots, x_n)| \le c_i,
$$
for constants $c_i, 1 \le i \le n$. Then for every $\epsilon > 0$,
% \begin{eqnarray*}
%     \mathrm{Pr}[f(X_1,\dots,X_n) - {\mathbb E}f(X_1,\dots,X_n) \ge \epsilon] & \le & \exp\left(\frac{-2\epsilon^2}{\sum_{i=1}^n c_i^2}\right),\;\mathrm{and}\\
%     \mathrm{Pr}[{\mathbb E}f(X_1,\dots,X_n) - f(X_1,\dots,X_n) \ge \epsilon] & \le & \exp\left(\frac{-2\epsilon^2}{\sum_{i=1}^n c_i^2}\right).
% \end{eqnarray*}
\begin{align*}
    \mathrm{Pr}[f - {\mathbb E}[f] \ge \epsilon] & \le \exp\left(\frac{-2\epsilon^2}{\sum_{i=1}^n c_i^2}\right),\;\mathrm{and}\\
    \mathrm{Pr}[{\mathbb E}[f] - f \ge \epsilon] & \le \exp\left(\frac{-2\epsilon^2}{\sum_{i=1}^n c_i^2}\right).
\end{align*}
\end{thm}

\begin{proof}[\bf Proof of Theorem 4]
From (16) and (17) and the symmetry of $d_\kappa(\cdot,\cdot)$, we have
\begin{eqnarray*}
    \hat{\Delta}_k & = & \frac{1}{n_k(n_k-1)} \sum_{i,j \in \mathcal{I}_k} d_\kappa(x_i,x_j), \\
    \hat{\Delta} & = & \frac{1}{n(n-1)} \sum_{i,j} d_\kappa(x_i,x_j).
\end{eqnarray*}
The proof is based on McDiarmid's inequality. We define
$$
f((x_1,y_1),\cdots,(x_n,y_n)) := \mathrm{gCov}_\kappa^n = \hat{\Delta} - \sum_k{\hat{p}_k\hat{\Delta}_k}.
$$
For a change of $(x_i,y_i)$ to $(\hat{x}_i,\hat{y}_i)$, the change of $f$ is denoted by 
% $$
% \delta f_i = f((x_1,y_1), \cdots,(x_i,y_i), \cdots,  (x_n,y_n)) - f((x_1,y_1), \cdots, (\hat{x}_i,\hat{y}_i), \cdots, (x_n,y_n)).
% $$
\begin{align*}
    &\delta f_i = f((x_1,y_1), \cdots,(x_i,y_i), \cdots,  (x_n,y_n))\\
    & - f((x_1,y_1), \cdots, (\hat{x}_i,\hat{y}_i), \cdots, (x_n,y_n)).
\end{align*}
Because of the symmetry of $f$, without loss of generality, we derive an upper bound for $\delta f_1$. The following two scenarios are considered.

Case 1: $\hat{y}_1 = y_1$.
% \begin{eqnarray*}
%     \delta f_1 & = & \sum_{i,j\ne 1}\frac{d_\kappa(x_i,x_j)}{n(n-1)} + \sum_{j} \frac{2d_\kappa(x_1,x_j)}{n(n-1)} - \sum_{i,j \in \mathcal{I}_1;i,j\ne 1} \frac{d_\kappa(x_i,x_j)}{n(n_1-1)} - \\
%     & & \sum_{j \in \mathcal{I}_1} \frac{2d_\kappa(x_1,x_j)}{n(n_1-1)} - \sum_{k>1}\sum_{i,j\in\mathcal{I}_k} \frac{d_\kappa(x_i,x_j)}{n(n_k-1)} - \\
%      & & \sum_{i,j\ne 1} \frac{d_\kappa(x_i,x_j)}{n(n-1)} - \sum_{j} \frac{2d_\kappa(\hat{x}_1,x_j)}{n(n-1)} + \sum_{i,j \in \mathcal{I}_1;i,j\ne 1} \frac{d_\kappa(x_i,x_j)}{n(n_1-1)} + \\
%      & & \sum_{j \in \mathcal{I}_1,} \frac{2d_\kappa(\hat{x}_1,x_j)}{n(n_1-1)} + \sum_{k>1}\sum_{i,j\in\mathcal{I}_k} \frac{d_\kappa(x_i,x_j)}{n(n_k-1)}\\
%      & = & \sum_{j}\frac{2\left[d_\kappa(x_1,x_j) - d_\kappa(\hat{x}_1,x_j) \right]}{n(n-1)} + \sum_{j\in\mathcal{I}_1} \frac{2\left[ d_\kappa(\hat{x}_1,x_j) - d_\kappa(x_1,x_j) \right]}{n(n_1-1)} \\
%      & \le & \frac{2}{n} + \frac{2}{n} = \frac{4}{n}.
% \end{eqnarray*}
\begin{align*}
    \delta f_1 & = \sum_{i,j\ne 1}\frac{d_\kappa(x_i,x_j)}{n(n-1)} + \sum_{j} \frac{2d_\kappa(x_1,x_j)}{n(n-1)} -  \\
    & \sum_{i,j \in \mathcal{I}_1;i,j\ne 1} \frac{d_\kappa(x_i,x_j)}{n(n_1-1)} - \sum_{j \in \mathcal{I}_1}  \frac{2d_\kappa(x_1,x_j)}{n(n_1-1)} - \\
    & \sum_{k>1}\sum_{i,j\in\mathcal{I}_k} \frac{d_\kappa(x_i,x_j)}{n(n_k-1)} - \sum_{i,j\ne 1} \frac{d_\kappa(x_i,x_j)}{n(n-1)} - \\
    & \sum_{j} \frac{2d_\kappa(\hat{x}_1,x_j)}{n(n-1)} + \sum_{i,j \in \mathcal{I}_1;i,j\ne 1} \frac{d_\kappa(x_i,x_j)}{n(n_1-1)} + \\
     & \sum_{j \in \mathcal{I}_1,} \frac{2d_\kappa(\hat{x}_1,x_j)}{n(n_1-1)} + \sum_{k>1}\sum_{i,j\in\mathcal{I}_k} \frac{d_\kappa(x_i,x_j)}{n(n_k-1)}\\
     & = \sum_{j}\frac{2\left[d_\kappa(x_1,x_j) - d_\kappa(\hat{x}_1,x_j) \right]}{n(n-1)} \\
     &+ \sum_{j\in\mathcal{I}_1} \frac{2\left[ d_\kappa(\hat{x}_1,x_j) - d_\kappa(x_1,x_j) \right]}{n(n_1-1)} \\
     & \le \frac{2}{n} + \frac{2}{n} = \frac{4}{n}.
\end{align*}

Case 2: $\hat{y}_1 = y_2$.
% \begin{eqnarray*}
%     \delta f_1 & = & \sum_{i,j\ne 1} \frac{d_\kappa(x_i,x_j)}{n(n-1)} + \sum_{j} \frac{2d_\kappa(x_1,x_j)}{n(n-1)} - \sum_{i,j \in \mathcal{I}_1; i,j \ne 1} \frac{d_\kappa(x_i,x_j)}{n(n_1-1)} - \\
%     & & \sum_{j \in \mathcal{I}_1} \frac{2d_\kappa(x_1,x_j)}{n(n_1-1)} - \sum_{i,j \in \mathcal{I}_2} \frac{d_\kappa(x_i,x_j)}{n(n_2-1)} - \sum_{k>2}\sum_{i,j\in\mathcal{I}_k} \frac{d_\kappa(x_i,x_j)}{n(n_k-1)} - \\
%     & & \sum_{i,j\ne 1} \frac{d_\kappa(x_i,x_j)}{n(n-1)} - \sum_{j} \frac{2d_\kappa(\hat{x}_1,x_j)}{n(n-1)} + \sum_{i,j \in \mathcal{I}_1;i,j\ne 1} \frac{d_\kappa(x_i,x_j)}{n(n_1-2)} + \\
%     & & \sum_{j \in \mathcal{I}_2} \frac{2d_\kappa(\hat{x}_1,x_j)}{n\cdot n_2} + \sum_{i,j \in \mathcal{I}_2} \frac{d_\kappa(x_i,x_j)}{n\cdot n_2} + \sum_{k>2}\sum_{i,j\in\mathcal{I}_k} \frac{d_\kappa(x_i,x_j)}{n(n_k-1)}\\
%     & = & \sum_{j}\frac{2\left[d_\kappa(x_1,x_j) - d_\kappa(\hat{x}_1,x_j) \right]}{n(n-1)} + \sum_{i,j \in \mathcal{I}_1;i,j\ne 1}\frac{d_\kappa(x_i,x_j)}{n(n_1-1)(n_1-2)} + \\
%     & & \sum_{j \in \mathcal{I}_2} \frac{2d_\kappa(\hat{x}_1,x_j)}{n\cdot n_2} - \sum_{j \in \mathcal{I}_1} \frac{2d_\kappa(x_1,x_j)}{n(n_1-1)} - \sum_{i,j\in \mathcal{I}_2}\frac{d_\kappa(x_i,x_j)}{n\cdot n_2(n_2-1)} \\
%     & \le & \frac{2}{n} + \frac{1}{n} + \frac{2}{n} = \frac{5}{n}.
% \end{eqnarray*}
\begin{align*}
    \delta f_1 & = \sum_{i,j\ne 1} \frac{d_\kappa(x_i,x_j)}{n(n-1)} + \sum_{j} \frac{2d_\kappa(x_1,x_j)}{n(n-1)} - \\
    &\sum_{i,j \in \mathcal{I}_1; i,j \ne 1} \frac{d_\kappa(x_i,x_j)}{n(n_1-1)} - \sum_{j \in \mathcal{I}_1} \frac{2d_\kappa(x_1,x_j)}{n(n_1-1)} - \\
    &\sum_{i,j \in \mathcal{I}_2} \frac{d_\kappa(x_i,x_j)}{n(n_2-1)} - \sum_{k>2}\sum_{i,j\in\mathcal{I}_k} \frac{d_\kappa(x_i,x_j)}{n(n_k-1)} - \\
    & \sum_{i,j\ne 1} \frac{d_\kappa(x_i,x_j)}{n(n-1)} - \sum_{j} \frac{2d_\kappa(\hat{x}_1,x_j)}{n(n-1)} + \\
    & \sum_{i,j \in \mathcal{I}_1;i,j\ne 1} \frac{d_\kappa(x_i,x_j)}{n(n_1-2)} + \sum_{j \in \mathcal{I}_2} \frac{2d_\kappa(\hat{x}_1,x_j)}{n\cdot n_2} + \\
    &\sum_{i,j \in \mathcal{I}_2} \frac{d_\kappa(x_i,x_j)}{n\cdot n_2} + \sum_{k>2}\sum_{i,j\in\mathcal{I}_k} \frac{d_\kappa(x_i,x_j)}{n(n_k-1)}\\
    & = \sum_{j}\frac{2\left[d_\kappa(x_1,x_j) - d_\kappa(\hat{x}_1,x_j) \right]}{n(n-1)} \\
    & + \sum_{i,j \in \mathcal{I}_1;i,j\ne 1}\frac{d_\kappa(x_i,x_j)}{n(n_1-1)(n_1-2)} + \sum_{j \in \mathcal{I}_2} \frac{2d_\kappa(\hat{x}_1,x_j)}{n\cdot n_2} \\ 
    & - \sum_{j \in \mathcal{I}_1} \frac{2d_\kappa(x_1,x_j)}{n(n_1-1)} - \sum_{i,j\in \mathcal{I}_2}\frac{d_\kappa(x_i,x_j)}{n\cdot n_2(n_2-1)} \\
    & \le \frac{2}{n} + \frac{1}{n} + \frac{2}{n} = \frac{5}{n}.
\end{align*}
Combining Cases $1$ and $2$, we have $|\delta f_i| \le \frac{5}{n}$ for $i=1,\cdots,n$. The proof is completed by applying McDiarmid's inequality with $c_i=\frac{5}{n}$.
\end{proof}

\begin{proof}[\bf Proof of Theorem 5]
From (17), we have
$$
\hat{\Delta} = \frac{1}{n(n-1)} \sum_{i,j} d_\kappa(x_i,x_j).
$$
We define $f(x_1,\cdots,x_n) :=\hat{\Delta}$ and 
$$
\delta f_i = f(x_1, \cdots,x_i, \cdots,  x_n) - f(x_1, \cdots, \hat{x}_i, \cdots, x_n)
$$
to be the change of $f$ for a change of $x_i$ to $\hat{x}_i$. Without loss of generality, we consider $\delta f_1$. It follows that
% \begin{eqnarray*}
%     \delta f_1 & = & \sum_{i,j\ne 1}\frac{d_\kappa(x_i,x_j)}{n(n-1)} + \sum_{j}\frac{2d_\kappa(x_1,x_j)}{n(n-1)} - \sum_{i,j\ne 1}\frac{d_\kappa(x_i,x_j)}{n(n-1)} - \sum_{j}\frac{2d_\kappa(\hat{x}_1,x_j)}{n(n-1)} \\
%     & = & \sum_{j}\frac{2\left[ d_\kappa(x_1,x_j) - d_\kappa(\hat{x}_1,x_j) \right]}{n(n-1)} \le \frac{2}{n}.
% \end{eqnarray*}
\begin{align*}
    \delta f_1 & = \sum_{i,j\ne 1}\frac{d_\kappa(x_i,x_j)}{n(n-1)} + \sum_{j}\frac{2d_\kappa(x_1,x_j)}{n(n-1)}  \\
    &- \sum_{i,j\ne 1}\frac{d_\kappa(x_i,x_j)}{n(n-1)} - \sum_{j}\frac{2d_\kappa(\hat{x}_1,x_j)}{n(n-1)} \\
    & = \sum_{j}\frac{2\left[ d_\kappa(x_1,x_j) - d_\kappa(\hat{x}_1,x_j) \right]}{n(n-1)} \le \frac{2}{n}.
\end{align*}
Applying McDiarmid's inequality with $c_i = \frac{2}{n}$ completes the proof.
\end{proof}

%you can choose not to have a title for an appendix if you want by leaving the argument blank
\section{Proof of the uniform convergence bound for generalized distance covariance}\label{app_c}
\begin{proof}
We will apply McDiarmid's inequality to establish the upper bound. Let
% $$
% f((x_1,y_1),\cdots,(x_n,y_n)) := \mathrm{dCov}_{\kappa_X,\kappa_y}^n = \frac{1}{n(n-3)}\sum_{i\ne j}A_{ij}B_{ij}.
% $$
\begin{align*}
    f((x_1,y_1),\cdots,(x_n,y_n)) &:= \mathrm{dCov}_{\kappa_X,\kappa_y}^n \\
                                  &= \frac{1}{n(n-3)}\sum_{i\ne j}A_{ij}B_{ij}.
\end{align*}
Similar to the proof of Theorem 4, for a change of $(x_i,y_i)$ to $(\Hat{x}_i,\hat{y}_i)$, the change on $f$ is denoted by $\delta f_i$.
% $$
% \delta f_i = f((x_1,y_1), \cdots,(x_i,y_i), \cdots,  (x_n,y_n)) - f((x_1,y_1), \cdots, (\hat{x}_i,\hat{y}_i), \cdots, (x_n,y_n)).
% $$
Due to symmetry of $f$, without loss of generality, we derive an upper bound for $|\delta f_1|$. The change of $(x_1,y_1)$ to $(\hat{x}_1,\Hat{y}_1)$ affects the following variables: $a_{1j}$, $a_{i1}$, $a_{i\cdot}$, $a_{\cdot j}$, $a_{\cdot \cdot}$, $b_{1j}$, $b_{i1}$, $b_{i\cdot}$, $b_{\cdot j}$, $b_{\cdot \cdot}$. We denote the changed variables as $\hat{a}_{1j}$, $\hat{a}_{i1}$, $\hat{a}_{i\cdot}$, $\hat{a}_{\cdot j}$, $\hat{a}_{\cdot \cdot}$, $\hat{b}_{1j}$, $\hat{b}_{i1}$, $\hat{b}_{i\cdot}$, $\hat{b}_{\cdot j}$, $\hat{b}_{\cdot \cdot}$, respectively. Two scenarios are considered.

Case $1$: $\left| A_{1j}B_{1j} - \hat{A}_{1j}\hat{B}_{1j} \right|$, $j\ne 1$. (Because of symmetric, the result holds for $\left| A_{i1}B_{i1} - \hat{A}_{i1}\hat{B}_{i1} \right|$, $i\ne 1$.)\\
Let
\begin{align*}
    A_{1j} & = a_{1j} - \frac{1}{n-2}a_{1\cdot} - \frac{1}{n-2}a_{\cdot 1} + \frac{1}{(n-1)(n-2)}a_{\cdot \cdot}, \\
    B_{1j} & = b_{1j} - \frac{1}{n-2}b_{1\cdot} - \frac{1}{n-2}b_{\cdot 1} + \frac{1}{(n-1)(n-2)}b_{\cdot \cdot}, \\
    \hat{A}_{1j} & = \hat{a}_{1j} - \frac{1}{n-2}\hat{a}_{1\cdot} - \frac{1}{n-2}\hat{a}_{\cdot 1} + \frac{1}{(n-1)(n-2)}\hat{a}_{\cdot \cdot}, \\
    \hat{B}_{1j} & = \hat{b}_{1j} - \frac{1}{n-2}\hat{b}_{1\cdot} - \frac{1}{n-2}\hat{b}_{\cdot 1} + \frac{1}{(n-1)(n-2)}\hat{b}_{\cdot \cdot},
\end{align*}
we have
% \begin{eqnarray*}
%     \left|A_{1j}B_{1j} - \hat{A}_{1j}\Hat{B}_{1j} \right| & \le & \left| A_{1j}B_{1j} \right| + \left| \hat{A}_{1j}\hat{B}_{1j} \right| \\
%     & = & \left|\left(a_{1j} - \frac{a_{1\cdot}}{n-2} - \frac{a_{\cdot j}}{n-2} + \frac{a_{\cdot \cdot}}{(n-1)} \right)\left(b_{1j} - \frac{b_{1\cdot}}{n-2} - \frac{b_{\cdot j}}{n-2} + \frac{b_{\cdot \cdot}}{(n-1)} \right) \right| + \\
%     & & \left|\left(\hat{a}_{1j} - \frac{\hat{a}_{1\cdot}}{n-2} - \frac{\hat{a}_{\cdot j}}{n-2} + \frac{\hat{a}_{\cdot \cdot}}{(n-1)} \right)\left(\hat{b}_{1j} - \frac{\hat{b}_{1\cdot}}{n-2} - \frac{\hat{b}_{\cdot j}}{n-2} + \frac{\hat{b}_{\cdot \cdot}}{(n-1)} \right) \right| \\
%     & \le & \left(\left|a_{1j} - \frac{a_{1\cdot}}{n-2} \right| + \left|\frac{a_{\cdot j}}{n-2} - \frac{a_{\cdot \cdot}}{(n-1)(n-2)} \right| \right) \\
%     & & \left(\left|b_{1j} - \frac{b_{1\cdot}}{n-2} \right| + \left|\frac{b_{\cdot j}}{n-2} - \frac{b_{\cdot \cdot}}{(n-1)(n-2)} \right| \right) + \\
%     &  & \left(\left|\hat{a}_{1j} - \frac{\hat{a}_{1\cdot}}{n-2} \right| + \left|\frac{\hat{a}_{\cdot j}}{n-2} - \frac{\hat{a}_{\cdot \cdot}}{(n-1)(n-2)} \right| \right) \\
%     &  & \left(\left|\hat{b}_{1j} - \frac{\hat{b}_{1\cdot}}{n-2} \right| + \left|\frac{\hat{b}_{\cdot j}}{n-2} - \frac{\hat{b}_{\cdot \cdot}}{(n-1)(n-2)} \right| \right) \\
%     & \le & \left(\frac{n-1}{n-2} + \frac{n}{n-2} \right)^2 + \left(\frac{n-1}{n-2} + \frac{n}{n-2} \right)^2 = 2\left( \frac{2n-1}{n-2}\right)^2.
% \end{eqnarray*}
\begin{align*}
    &\left|A_{1j}B_{1j} - \hat{A}_{1j}\Hat{B}_{1j} \right| \\
    & \le \left| A_{1j}B_{1j} \right| + \left| \hat{A}_{1j}\hat{B}_{1j} \right| \\
    % & = \left|\left(a_{1j} - \frac{a_{1\cdot}}{n-2} - \frac{a_{\cdot j}}{n-2} + \frac{a_{\cdot \cdot}}{(n-1)} \right)\left(b_{1j} - \frac{b_{1\cdot}}{n-2} - \frac{b_{\cdot j}}{n-2} + \frac{b_{\cdot \cdot}}{(n-1)} \right) \right| + \\
    % & \left|\left(\hat{a}_{1j} - \frac{\hat{a}_{1\cdot}}{n-2} - \frac{\hat{a}_{\cdot j}}{n-2} + \frac{\hat{a}_{\cdot \cdot}}{(n-1)} \right)\left(\hat{b}_{1j} - \frac{\hat{b}_{1\cdot}}{n-2} - \frac{\hat{b}_{\cdot j}}{n-2} + \frac{\hat{b}_{\cdot \cdot}}{(n-1)} \right) \right| \\
    & \le \left(\left|a_{1j} - \frac{a_{1\cdot}}{n-2} \right| + \left|\frac{a_{\cdot j}}{n-2} - \frac{a_{\cdot \cdot}}{(n-1)(n-2)} \right| \right) \\
    & \left(\left|b_{1j} - \frac{b_{1\cdot}}{n-2} \right| + \left|\frac{b_{\cdot j}}{n-2} - \frac{b_{\cdot \cdot}}{(n-1)(n-2)} \right| \right) + \\
    &  \left(\left|\hat{a}_{1j} - \frac{\hat{a}_{1\cdot}}{n-2} \right| + \left|\frac{\hat{a}_{\cdot j}}{n-2} - \frac{\hat{a}_{\cdot \cdot}}{(n-1)(n-2)} \right| \right) \\
    &  \left(\left|\hat{b}_{1j} - \frac{\hat{b}_{1\cdot}}{n-2} \right| + \left|\frac{\hat{b}_{\cdot j}}{n-2} - \frac{\hat{b}_{\cdot \cdot}}{(n-1)(n-2)} \right| \right) \\
    & \le \left(\frac{n-1}{n-2} + \frac{n}{n-2} \right)^2 + \left(\frac{n-1}{n-2} + \frac{n}{n-2} \right)^2 = 2\left( \frac{2n-1}{n-2}\right)^2.
\end{align*}

Case $2$: $\left| A_{ij}B_{ij} - \hat{A}_{ij}\hat{B}_{ij} \right|$, $i\ne j \ne 1$.\\
Let $\hat{A}_{ij} = A_{ij} + \delta_{ij}^a$ and $\hat{B}_{ij} = B_{ij} + \delta_{ij}^b$ where
\begin{align*}
    \delta_{ij}^a & = \frac{a_{i1} - \hat{a}_{i1}}{n-2} + \frac{a_{1j} - \hat{a}_{1j}}{n-2} + \frac{\sum_{k=2}^n{\left[\hat{a}_{1k} + \hat{a}_{k1} - a_{1k} - a_{k1}\right] }}{(n-1)(n-2},\\
    \delta_{ij}^b & = \frac{b_{i1} - \hat{b}_{i1}}{n-2} + \frac{b_{1j} - \hat{b}_{1j}}{n-2} + \frac{\sum_{k=2}^n{\left[\hat{b}_{1k} + \hat{b}_{k1} - b_{1k} - b_{k1}\right] }}{(n-1)(n-2},
\end{align*}
and
\begin{align*}
    \left| \delta_{ij}^a\right| & \le \frac{1}{n-2} + \frac{1}{n-2} + \frac{2}{n-2} = \frac{4}{n-2}, \\
    \left| \delta_{ij}^b\right| & \le \frac{1}{n-2} + \frac{1}{n-2} + \frac{2}{n-2} = \frac{4}{n-2}.
\end{align*}
Therefore,
% \begin{eqnarray*}
%     \left|A_{ij}B_{ij} - \hat{A}_{ij}\hat{B}_{ij} \right| & = & \left| A_{ij}B_{ij} - \left(A_{ij} + \delta_{ij}^a \right) \left(B_{ij} + \delta_{ij}^b \right) \right| \\
%     & = & \left| A_{ij} \delta_{ij}^b + B_{ij} \delta_{ij}^a + \delta_{ij}^a \delta_{ij}^b \right| \\
%     & \le & \left| A_{ij} \delta_{ij}^b \right| \left| B_{ij} \delta_{ij}^a \right| \left| \delta_{ij}^a \delta_{ij}^b \right| \\
%     & \le & \left(\frac{n-1}{n-2} + \frac{n}{n-2} \right)\frac{4}{n-2} + \left(\frac{n-1}{n-2} + \frac{n}{n-2} \right)\frac{4}{n-2} + \frac{16}{(n-2)^2}\\
%     & = & \frac{8(2n+1)}{(n-2)^2}.
% \end{eqnarray*}
\begin{align*}
    \left|A_{ij}B_{ij} - \hat{A}_{ij}\hat{B}_{ij} \right| & = \left| A_{ij}B_{ij} - \left(A_{ij} + \delta_{ij}^a \right) \left(B_{ij} + \delta_{ij}^b \right) \right| \\
    & = \left| A_{ij} \delta_{ij}^b + B_{ij} \delta_{ij}^a + \delta_{ij}^a \delta_{ij}^b \right| \\
    & \le \left| A_{ij} \delta_{ij}^b \right| \left| B_{ij} \delta_{ij}^a \right| \left| \delta_{ij}^a \delta_{ij}^b \right| \\
    & \le \left(\frac{n-1}{n-2} + \frac{n}{n-2} \right)\frac{4}{n-2} \\
    &+ \left(\frac{n-1}{n-2} + \frac{n}{n-2} \right)\frac{4}{n-2} + \frac{16}{(n-2)^2}\\
    & = \frac{8(2n+1)}{(n-2)^2}.
\end{align*}
Among all $A_{ij}B_{ij} - \hat{A}_{ij}\hat{B}_{ij}$, there are $2(n-1)$ instances of Case $1$ and $(n-1)(n-2)$ instances of Case $2$. Therefore,
% \begin{eqnarray*}
%     \left| \delta f_1 \right| & \le & \frac{1}{n(n-3)}\sum_{i\ne j} \left| A_{ij}B_{ij} - \hat{A}_{ij} \hat{B}_{ij}\right|\\
%     & \le & \frac{1}{n(n-3)}\left[2(n-1)\times 2 \left(\frac{2n-1}{n-2}\right)^2 + (n-1)(n-2)\frac{8(2n+1)}{(n-2)^2}\right] \\
%     & = & \frac{4(n-1)(2n-3)(4n+1)}{n(n-3)(n-2)^2} < \frac{32}{n}.
% \end{eqnarray*}
\begin{align*}
%\begin{split}
    \left| \delta f_1 \right| & \le \frac{1}{n(n-3)}\sum_{i\ne j} \left| A_{ij}B_{ij} - \hat{A}_{ij} \hat{B}_{ij}\right|\\
    & \le \frac{1}{n(n-3)}\left[2(n-1)\times 2 \left(\frac{2n-1}{n-2}\right)^2\right. \\
    &\left.+ (n-1)(n-2)\frac{8(2n+1)}{(n-2)^2}\right] \\
    & = \frac{4(n-1)(2n-3)(4n+1)}{n(n-3)(n-2)^2} < \frac{32}{n}.
% \end{split}
\end{align*}
Applying McDiarmid's inequality with $c_i=\frac{32}{n}$ completes the proof.
\end{proof}

% Can use something like this to put references on a page
% by themselves when using endfloat and the captionsoff option.
\ifCLASSOPTIONcaptionsoff
  \newpage
\fi

\end{document}
